# Supplementary material for: Slow and steady feature analysis: higher order temporal coherence in video
Source: arXiv:1506.04714 source file (2016-04-14)

# KITTI driving video

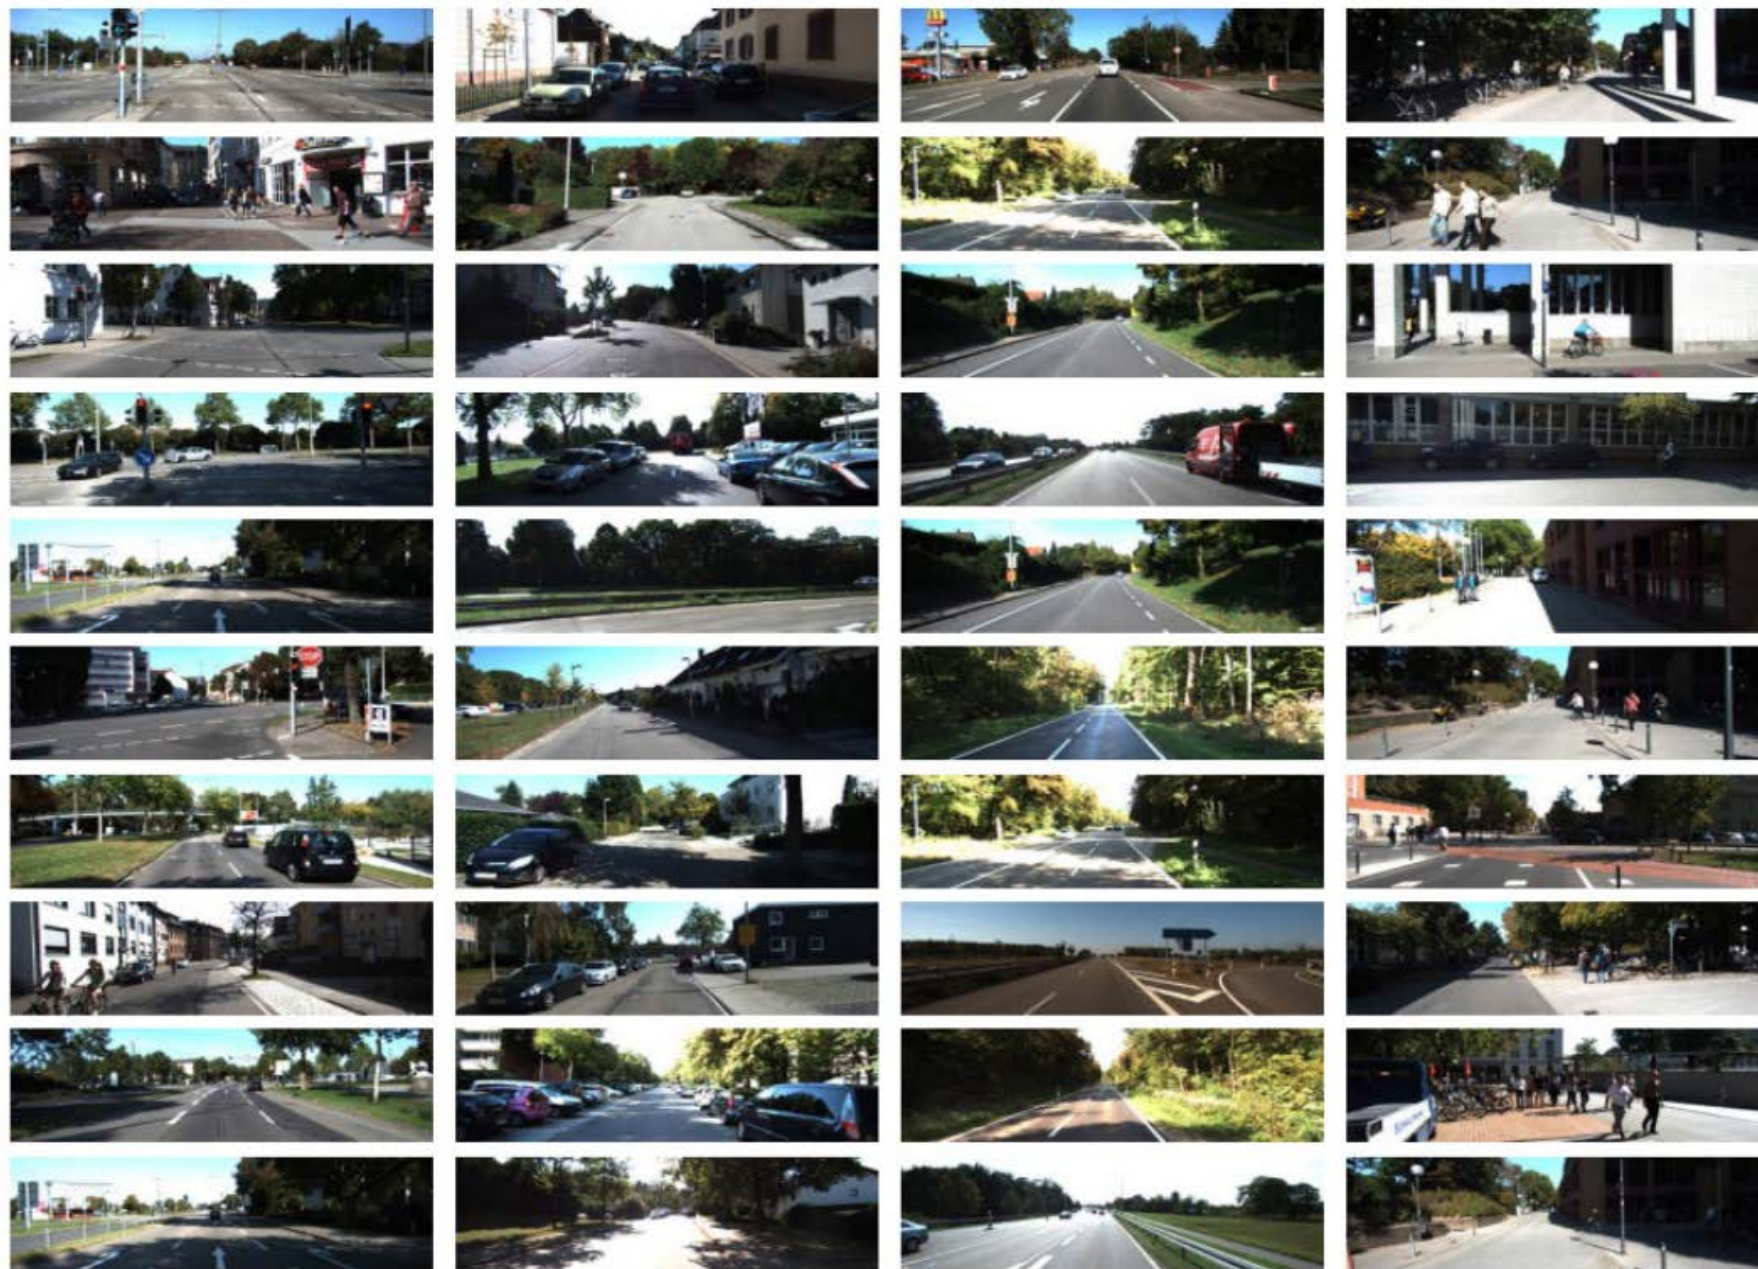

City

Residential

Road

Campus



# SUN scene images

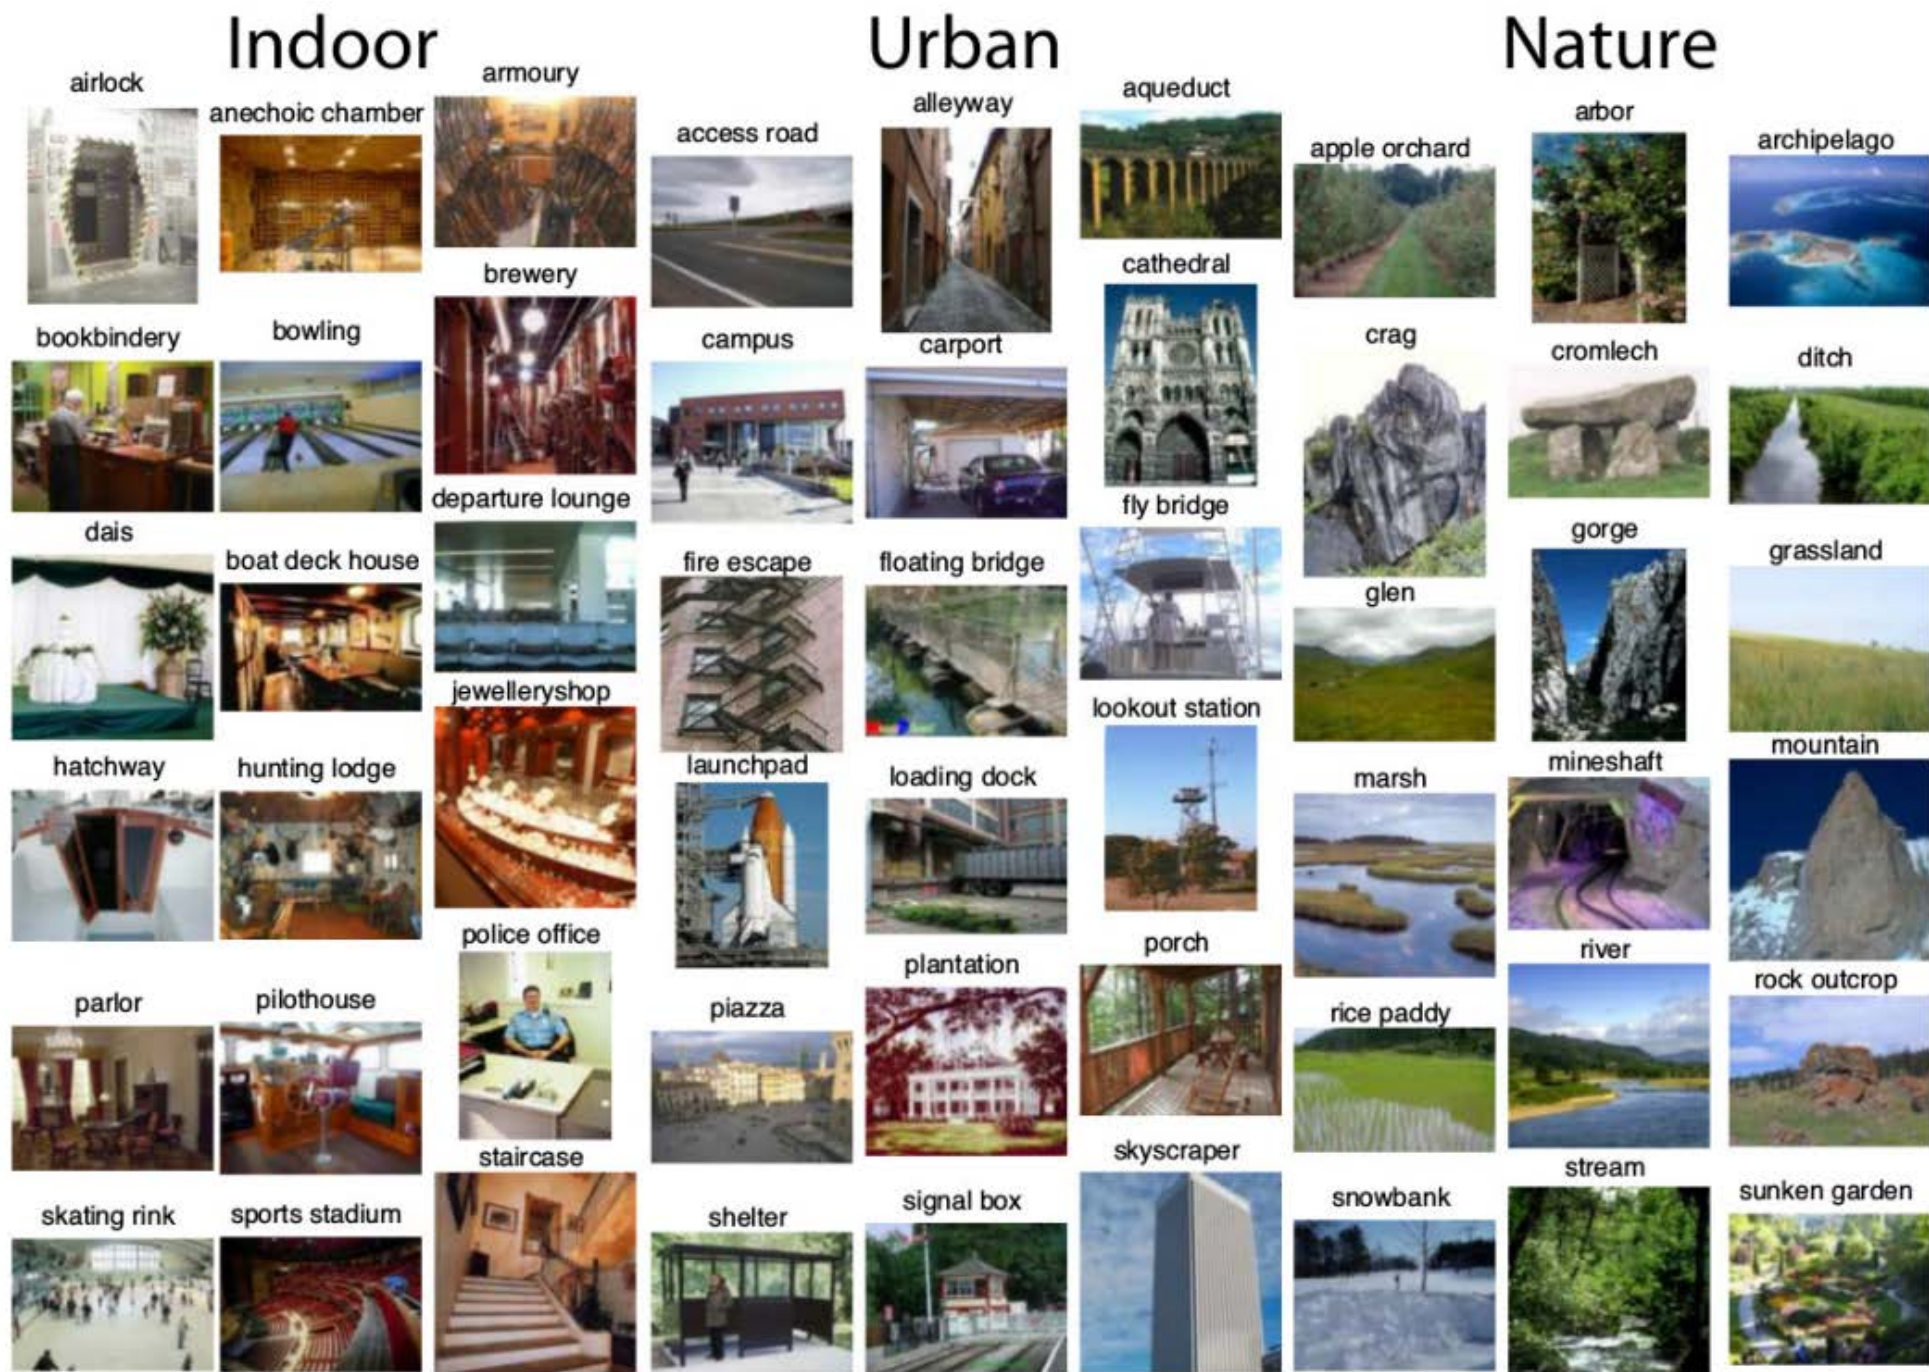



# HMDB-51 actions video

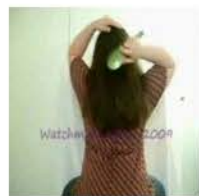

brush  
hair

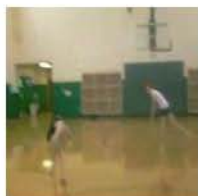

cartwheel

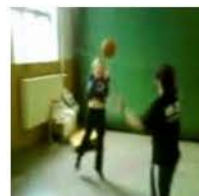

catch

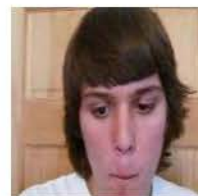

chew

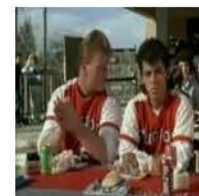

clap

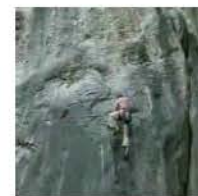

climb

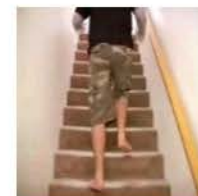

climb  
stairs

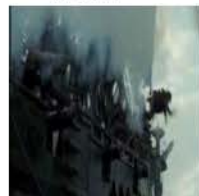

dive

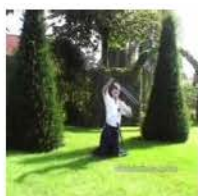

draw  
sword

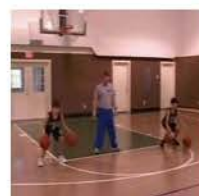

dribble

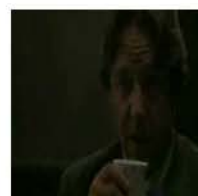

drink

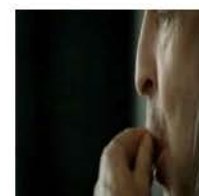

eat

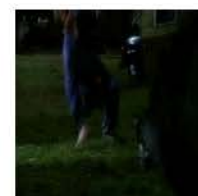

fall  
floor

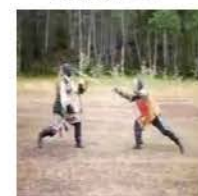

fencing

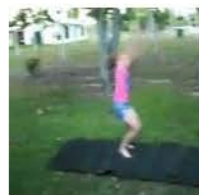

flic  
flac

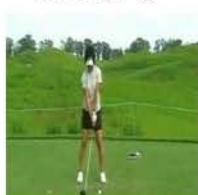

golf

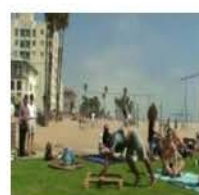

hand  
stand

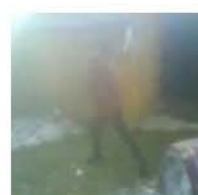

hit

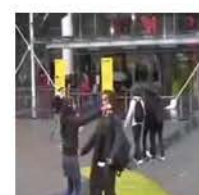

hug

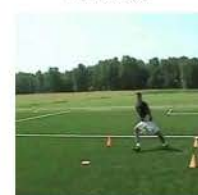

jump

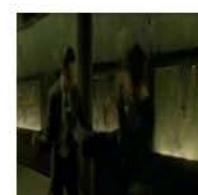

kick

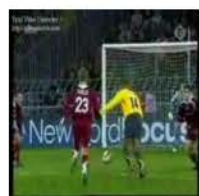

kick  
ball

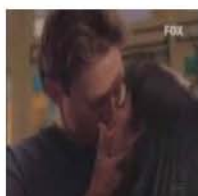

kiss

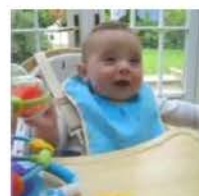

laugh

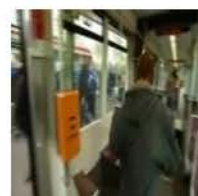

pick

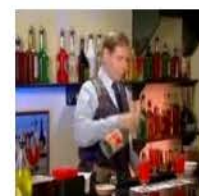

pour

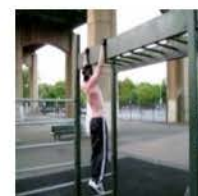

pullup

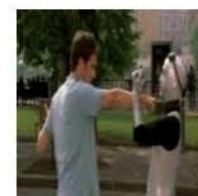

punch



# PASCAL-10 action still images

Phoning

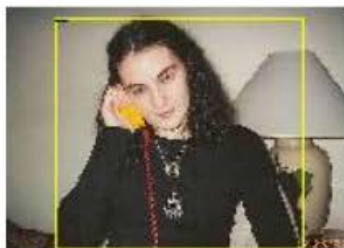

Playing Instrument

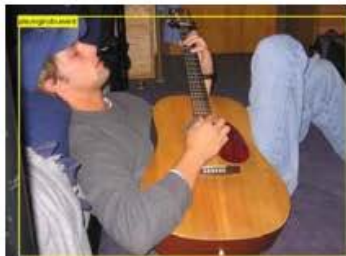

Reading

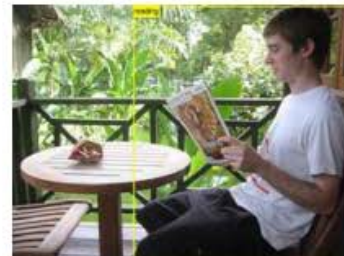

Riding Bike

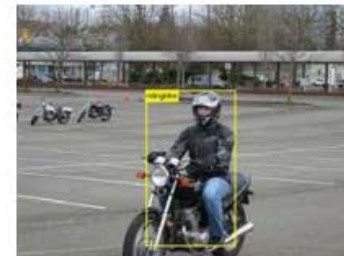

Riding Horse

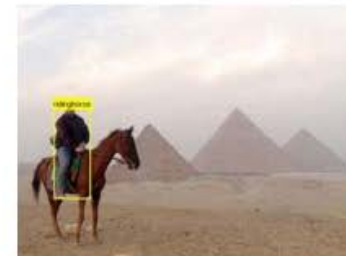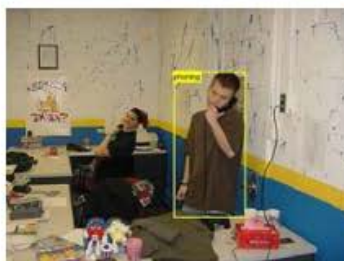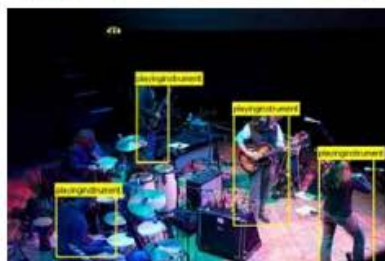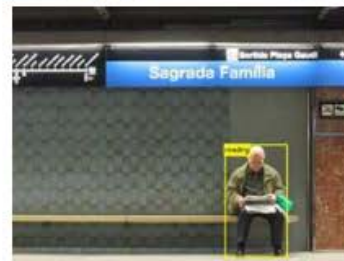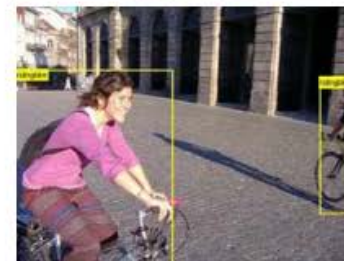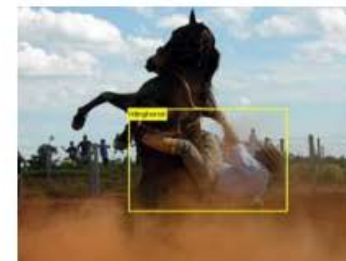

Running

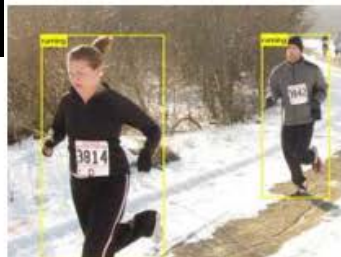

Taking Photo

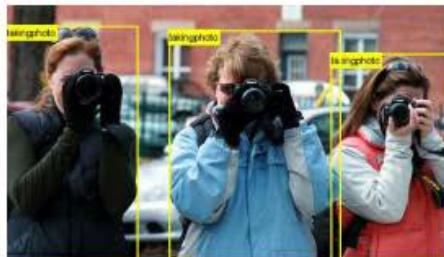

Using Computer

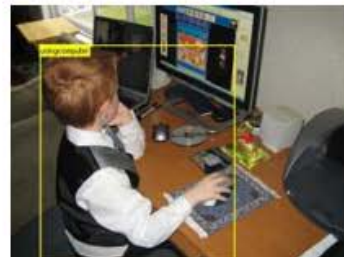

Walking

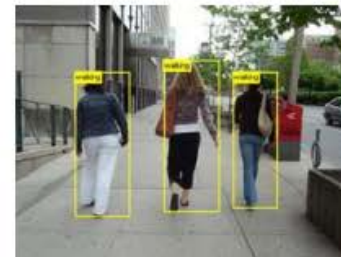

Jumping

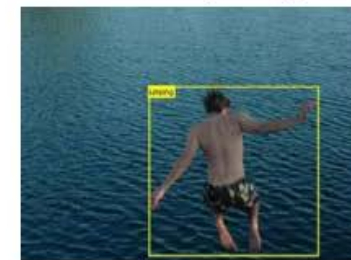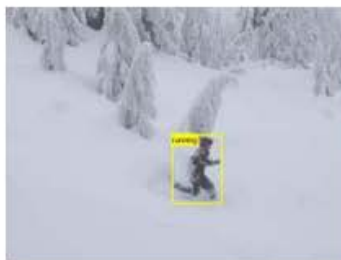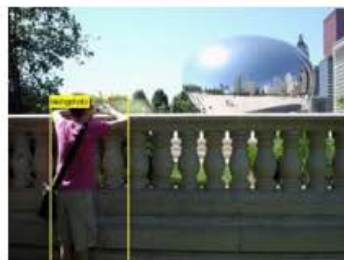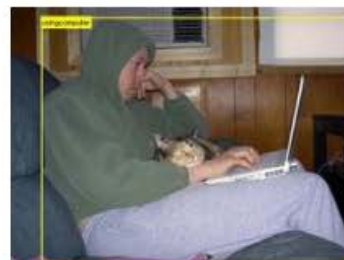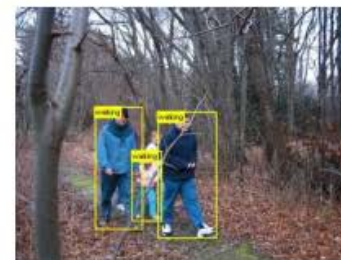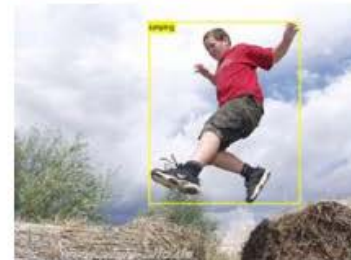

Supplement: Supplementary file 1 [file datasets-supp.pdf]
